# Supplementary material for: Eigenmodes of the Laplacian on Hyperbolic Lattices
Source: arXiv:2306.08248 source file (2024-04-22)
Supplement: Supplementary file 1 [file supplement.tex]

%=====================================================
% Eigenmodes of the Laplacian on Hyperbolic Lattices
% Supplemental Material
%=====================================================

\newpage
\onecolumngrid

\section{Supplemental Material}

%=====================================================
\subsection{S1: Hyperbolic Plane-Wave Eigenfunctions in the Continuum}
\label{sec:S1}
%=====================================================

To comprehend the analog of a plane wave on the Poincaré disk in the continuum case, we should initially revisit the situation in the Euclidean $\mathbb R^n$. Here the plane-wave solutions of the eigenvalue problem $\Delta \psi = -\lambda \psi$ are given by $\psi_{\vec k}(\vec x) = e^{i \vec k \cdot \vec x}$, where $\vec k \in \mathbb R^n$ denotes the momentum vector and $\lambda = k^2$ is the corresponding eigenvalue. Using the Euclidean distance $d(\vec x,\vec y)=||\vec x-\vec y||$, it can be shown that these eigenfunctions can be expressed in terms of the limit
\begin{equation}
\psi_{\vec k}(\vec x) =
e^{i \vec k \cdot \vec x} =
\lim_{r \to \infty} e^{-ik\bigl( d(\vec x, r \vec k)-d(0, r \vec k) \bigr)} \,,
\end{equation}
where $r \vec k$ is a point approaching infinity in the direction of $\vec k$. This elucidates that a plane wave can be perceived as a radial wave originating from a specific point at infinity.

We can apply the same rationale to construct the analogue of plane waves on the Poincaré disk. The only requirement is to replace the Euclidean distance by the geodesic distance
\begin{equation}
\text{d}(z,z') \;=\; \frac12\, \text{arcosh}\Bigl( 1+\frac{2|z-z'|^2}{(1-|z|^2)(1-|z'|^2)} \Bigr) \,.
\end{equation}
Note that points at infinity are now residing on the boundary of the disk $\partial \mathbb D$ where $|z|=1$. This suggests that we should define the hyperbolic equivalent of a plane wave on the Poincaré disk as
\begin{equation}
\psi_{\kappa,b}(z) \;:=\; \lim_{r \to 1} e^{-i\kappa\bigl( d(z,rb)-d(0,rb) \bigr)}\,.
\end{equation}
Here, $b = e^{i\beta}\in\partial\mathbb D$ is a point on the boundary of the disk, which we refer to as the \textit{source} of the plane wave in our study. Expanding the difference of the distance functions around $r=1$ leads to
\begin{equation}
\lim_{r \to 1}\bigl( d(z,rb)-d(0,rb) \bigr)\;=\;\frac12 \ln \frac{\bigl|z-b\bigr|^2}{1-|z|^2}
\end{equation}
and consequently,
\begin{equation}
\psi_{\kappa,b}(z) \;=\; \Bigl( \frac{1-|z|^2}{|1-z \overline b|^2} \Bigr)^{i\kappa/2}\,.
\end{equation}
By applying the Laplace-Beltrami operator $\Delta_g = 4(1-z\overline z)^2\partial_z \partial_{\overline z}$, it can be verified that this function solves the eigenvalue problem $\Delta_g \psi_{\kappa,b}=-\lambda \psi_{\kappa,ba}$. However, the corresponding eigenvalue $\lambda=\kappa(\kappa+2i)$ turns out to be complex-valued. To acquire a real positive spectrum with normalizable oscillatory eigenfunctions as in the Euclidean case, it is therefore useful to redefine the parameter $\kappa$ as $k=\kappa + i$, enabling us to interpret $k$ as a generalized momentum. This process results in the commonly accepted definition of hyperbolic plane waves in the literature~\cite{boettcher2020quantum}, specifically,
\begin{equation}
\psi_{k,b}(z) = \Bigl( \frac{1-|z|^2}{|1-z e^{-i\beta}|^2} \Bigr)^{\frac12(1+ik)}
\end{equation}
corresponding to the eigenvalue $\lambda=1+k^2$. These eigenfunctions deviate from Euclidean plane waves in that they demonstrate an additional exponential damping, as well as a constant offset in the eigenvalue, which is a consequence of the constant negative curvature of the hyperbolic space.

\begin{figure}[t]
\includegraphics[width=120mm]{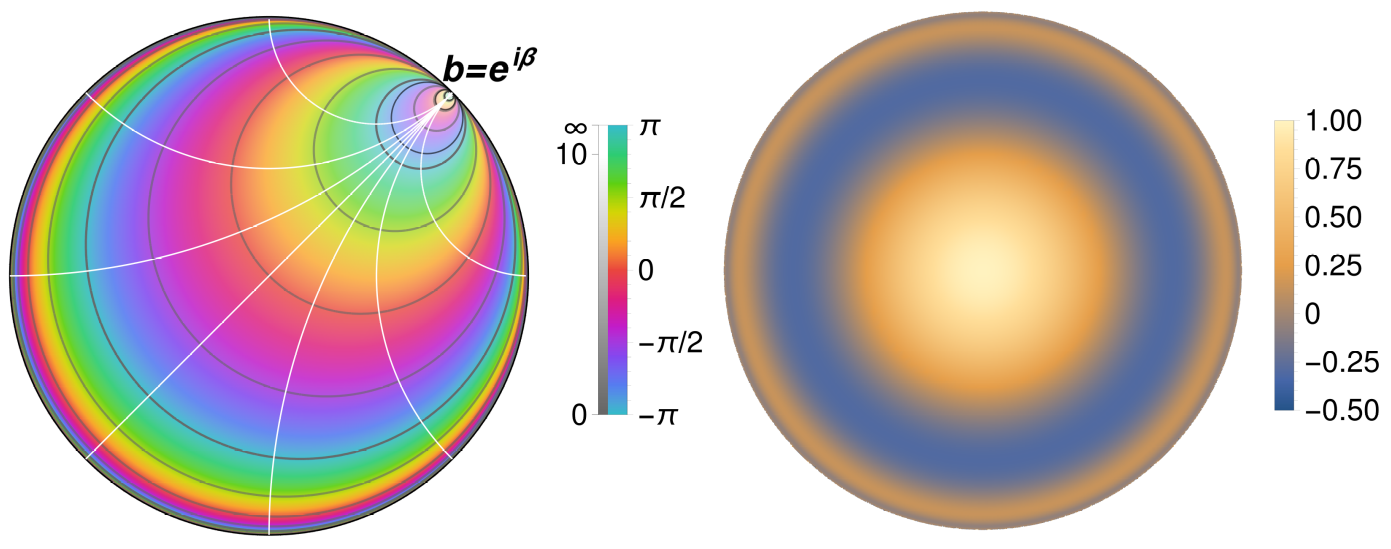}
\caption{Continuum eigenfunctions on the Poincaré disk. Left: Plane wave eigenfunction $\psi_{k,b}(z)$ for $\beta=\pi/4$ and $k=4$. The geodesics and horocycles are depicted as white and black circles, respectively. Right: The corresponding radial eigenfunction $u_{k}^m(z)$ for $m=0$.
\label{supfig:Eigensolutions}}
\end{figure}

Note that the eigenvalue $\lambda=1+k^2$ does not depend on the location of the source on the boundary. Therefore, the corresponding radial eigenfunctions can be obtained by a Fourier transformation in the angle $\beta$:
\begin{equation}
u_k^m(z) \;:=\;\frac{1}{2\pi} \int_0^{2\pi} \textrm{d}\beta \, e^{i m \beta}\psi_{k,e^{i \beta}}  \;\propto\; e^{i m \phi} P^m_{-\frac12(1+i k)}\Bigl( \frac{1+r^2}{1-r^2} \Bigr)\,,
\end{equation}
where $z=r e^{i\phi}$ and $P_\ell^m$ denote the associated Legendre functions. Examples of the plane wave solutions and the corresponding radial solutions are shown in Fig.~\ref{supfig:Eigensolutions}.

%=====================================================
\subsection{S2: Calculation of the Inclination at a given Vertex}
\label{sec:S2}
%=====================================================

In this section we present technical specifics  involved in computing the inclination, denoted as $\tau_j$, at a particular vertex of the hyperbolic lattice situated at the position  $z_j\in\mathbb D$. Let us assume that the source of the plane-wave eigenfunction resides at $b=e^{i\beta}\in\partial\mathbb D$ and that a geodesic line originating from $b$ intersects $z_j$, as depicted in Fig. 1 of the main text. Furthermore, let us denote the indices of the adjacent vertices by $j_0,j_1,\ldots,j_{q-1}$. This means that the neighboring vertices are located at the positions are located at the positions $z_{j_0},z_{j_1},\ldots,z_{j_{q-1}}$, as represented in Fig.~\ref{fig:taucalc}. Let us now apply the isometry
\begin{equation}
\label{SpecialIsometry}
z \mapsto w(z)=\frac{(1-b\overline z_j)(z-z_j)}{(b-z_j)(1-z\overline z_j)}\,,
\end{equation}
which maps the source at $b \in \partial \mathbb D$ to $1$ and the vertex at $z_j$ to the disk's center. As depicted in the figure, the new positions of the nearest neighbors, denoted as $w_n$, are then uniformly distributed along a circle
\begin{equation}
\label{DefWn}
w_n \;=\; w(z_{j_n}) \;=\; h \, e^{i(\alpha_j + 2\pi n/q)}\qquad \qquad (n=0,\ldots,q-1)
\end{equation}
with the radius $h$ given by
\begin{equation}
\label{hdef2}
h \;=\; \Bigl(1-\frac{\sin^2 (\pi/q)}{\cos^2 (\pi/p)}\Bigr)^{1/2}\,.
\end{equation}
Moreover, as illustrated in the right panel of the figure, the $q$ edges are now straight and form a regular star, which is angled against the horizontal geodesic line by the angle $\alpha_j$. Thus, we can deduce that $\alpha_j$ is defined by
\begin{equation}
e^{i q \alpha_j}\;=\;\Bigl(\frac{w_n}{h}  \Bigr)^q\,,
\end{equation}
where the choice of the neighbor labeled by $n=0,\ldots,q-1$ becomes irrelevant since it drops out when taking the $q^\textrm{th}$ power. Therefore, we can select just one  neighbor $j'=j_n$ of the vertex $j$ and denote its coordinate as $z'_j$. Since we have defined the \textit{inclination} as $\tau_j = \frac{q}{2\pi}\alpha_j$, we arrive at
\begin{equation}
\label{inclinationRelation}
e^{2\pi i \tau_j} \;=\; \Bigl( \frac 1 h \, \frac{(1-b \overline z_j)(z'_j-z_j)}{(b-z_j)(1-z'_j\overline z_j)} \Bigr)^q\,,
\end{equation}
where the square bracket encapsulates a complex number on the unit circle. Taking the argument allows us to disregard the factor $\frac{1}{h}$, leading to the final expression
\begin{equation}
\tau_j \;=\; \left(\frac{1}{2\pi} \arg \Bigl[\Bigl( \frac{(1-b \overline z_j)(z'_j-z_j)}{(b-z_j)(1-z'_j\overline z_j)} \Bigr)^q\Bigr]\right) \mod 1\,.
\end{equation}
In practice, once we have generated a hyperbolic tiling with vertex coordinates $z_j$ and defined the location of the source $b \in \partial \mathbb D$, we can compute the inclination parameter $\tau_j$ at every vertex $j$ of the infinite lattice simply by choosing one of its nearest neighbors $j'$ and employing the formula presented above.

\begin{figure}[t]
\centering\includegraphics[width=90mm]{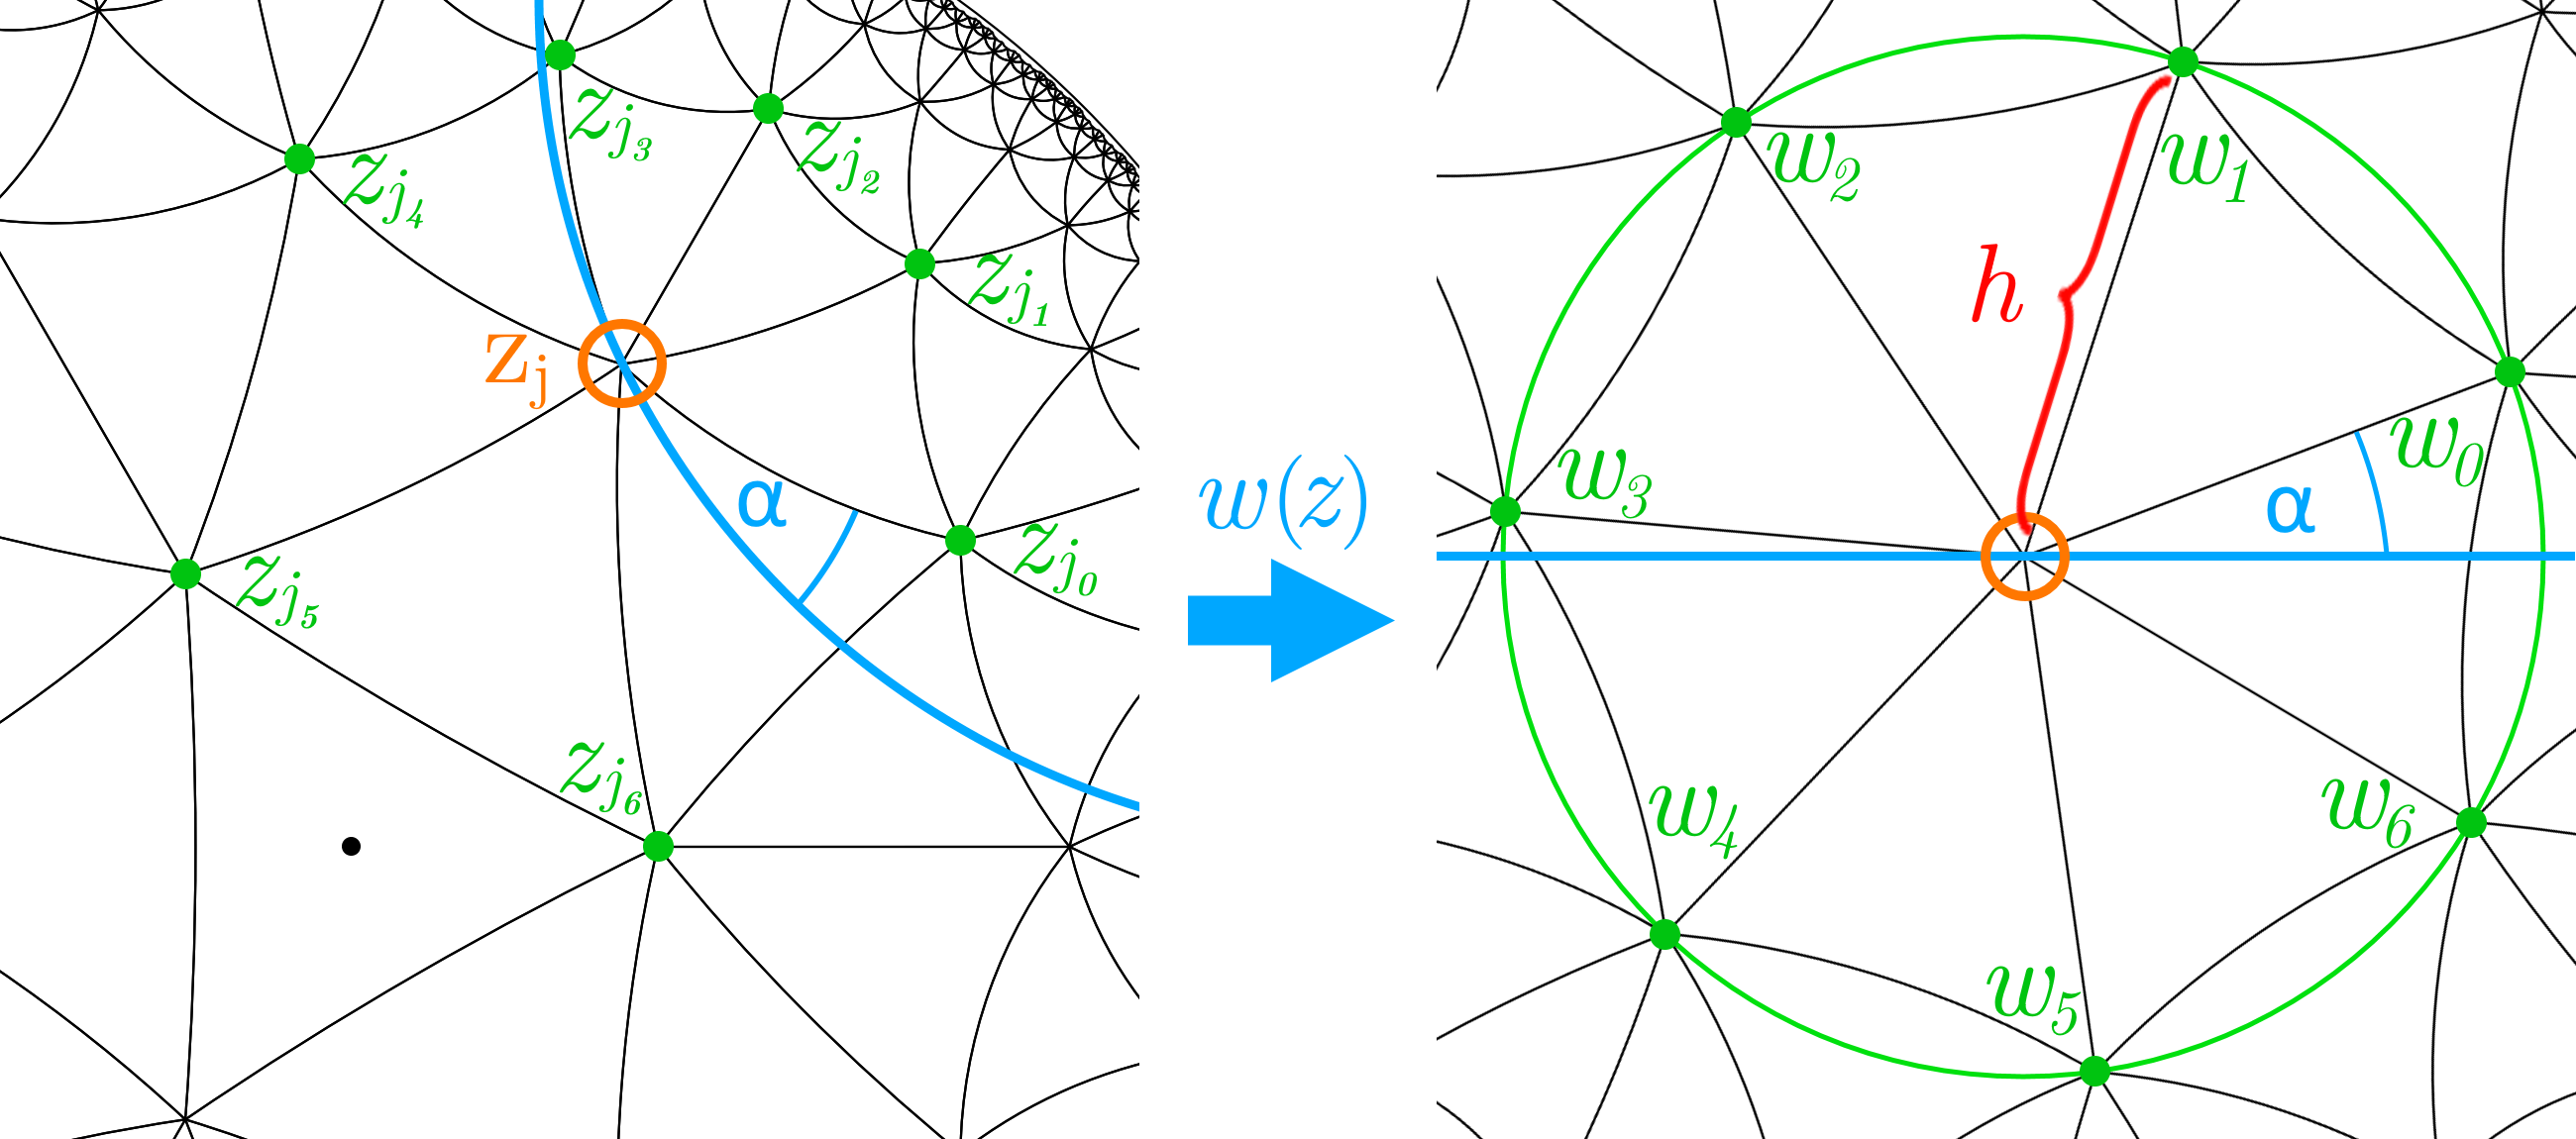}
\caption{
\label{fig:taucalc}
Mapping the cell with the vertex $j$ to the center in the example of a $\{3,7\}$-lattice.
}
\end{figure}

%=====================================================
\subsection{S3: Derivation of the non-local Difference Equation for the Correction Function $\chi(\tau)$}\label{sec:S3}
%=====================================================

In this section we derive the difference equation for the correction function, denoted as $\chi(\tau)$. Our starting point is the eigenvalue problem on the hyperbolic $\{p,q\}$-lattice provided in the main text:
\begin{equation}
\label{EigenvalueProblem}
\Delta^{\{p,q\}}\Psi_{\mu,b}(z_j) \;=\; -\Lambda_\mu\Psi_{\mu,b}(z_j)\,.
\end{equation}
Here, the hyperbolic lattice Laplacian $\Delta^{\{p,q\}}$ is defined in terms of the adjacency matrix $A_{jk}$:
\begin{equation}
\Delta^{\{p,q\}}\Psi_{\mu,b}(z_j) \;=\; \frac{1}{\mathcal N}\sum_k\Bigl( A_{jk}-q\delta_{jk} \Bigr)\Psi_{\mu,b}(z_k)\,,
\end{equation}
where $\mathcal N = \frac14 q h^2$ is a normalization factor. Utilizing the abbreviations $\Psi_j:=\Psi_{\mu,b}(z_j)$, we can recast the eigenvalue problem (\ref{EigenvalueProblem}) as follows:
\begin{equation}
\sum_k A_{jk}\Psi_k \;=\; \bigl(q-\mathcal N \Lambda_\mu\bigr) \Psi_j\,.
\end{equation}
As explicated in the main text, we assume that the lattice eigenfunctions $\Psi_j$  differ from the continuum eigenfunctions by a correction factor, i.e., we assume that
$$\Psi_j=\psi_j\chi_j\,,$$
where
\begin{equation}
\label{ContinuumEigenfunction}
\psi_j :=\psi_{\mu,b}(z_j) = \left( \frac{|b-z_j|^2}{1-|z_j|^2} \right)^{\mu}
\end{equation}
is the continuum eigenfunction and $\chi_j$ is a correction factor we aim to determine. This turns the eigenvalue problem into $\sum_k A_{jk}\psi_k\chi_k = (q-\mathcal N \Lambda_\mu) \psi_j\chi_j$. Since $\psi_j\neq 0$, we can divide by $\psi_j$, yielding an equivalent eigenvalue problem for the corrections $\chi_j$:
\begin{equation}
\label{EigenvalueProblem1}
\sum_k A_{jk}\frac{\psi_k}{\psi_j}\chi_k \;=\;
\sum_{n=0}^{q-1} R_{j,n}\,\chi_{j_n} \;=\;
\bigl(q-\mathcal N \Lambda_\mu\bigr) \chi_j\,.
\end{equation}
Here, we have defined
\begin{equation}
R_{j,n} \;:=\; \frac{\psi_{j_{n}}}{\psi_{j}}
\end{equation}
as the ratio of the continuum eigenfunctions. It can be shown that this ratio is an isometric invariant, i.e., it remains unaltered under any isometry of the form $z \mapsto w(z)=e^{i\eta}\tfrac{a-z}{1-z \overline a}$:
\begin{equation}
R_{j,n} \;=\;\frac{\psi_{j_n}}{\psi_j}\;=\;\frac{\psi_{\mu,b}(z_{j_n})}{\psi_{\mu,b}(z_j)}\;=\; \frac{\psi_{\mu,w(b)}(w(z_{j_n}))}{\psi_{\mu,w(b)}(w(z_j))}\,.
\end{equation}
\begin{figure}[t]
\includegraphics[width=90mm]{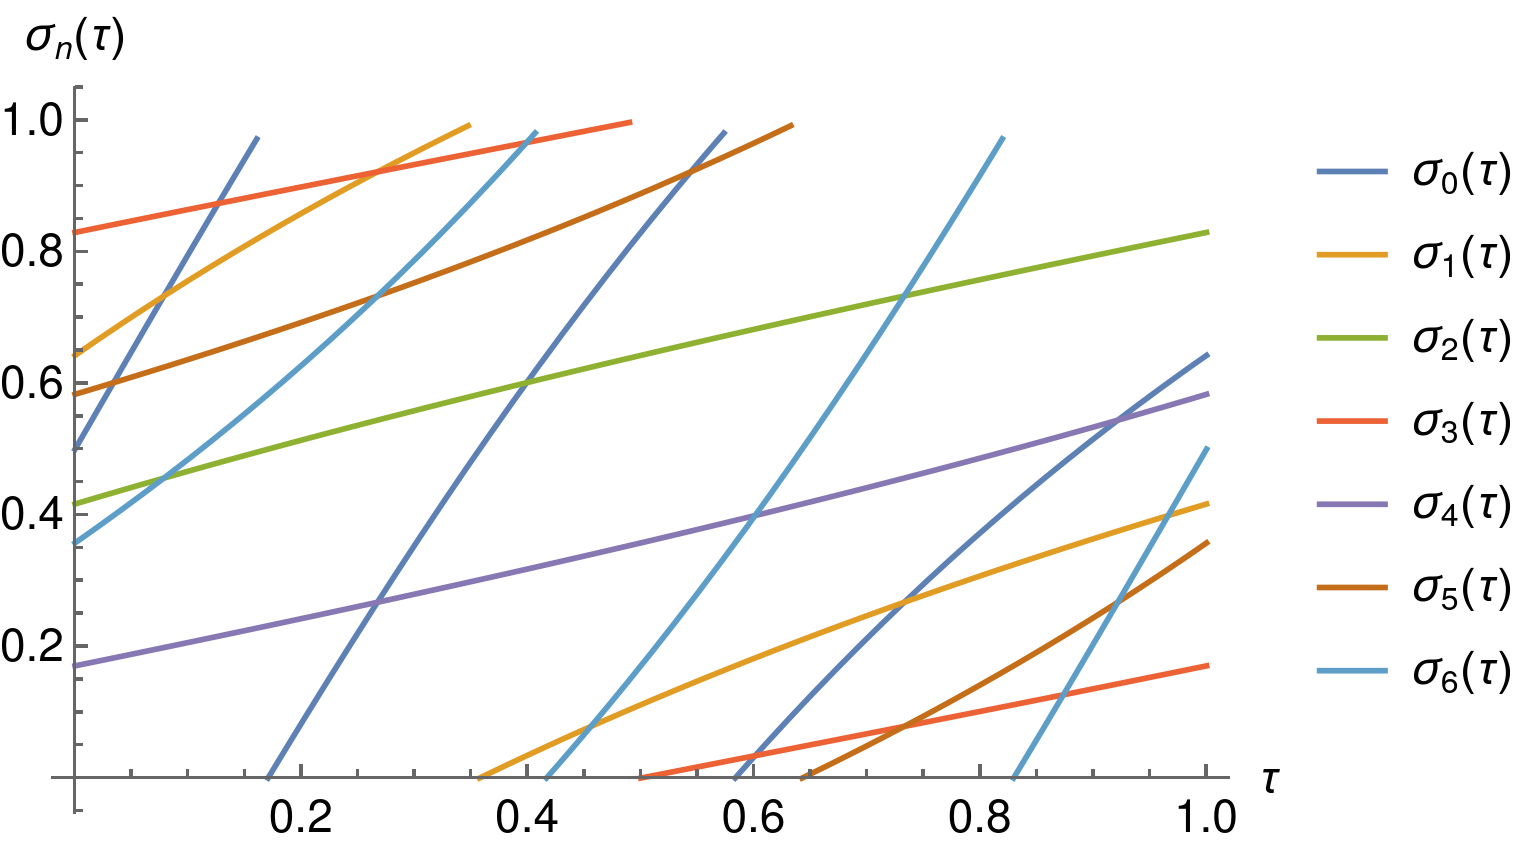}
\caption{Inclination $\sigma_n(\tau)$ of the $n^\text{th}$ neighbor of a vertex with inclination $\tau$ on a $\{3,7\}$ lattice.
\label{supfig:neighbor-inclination}}
\end{figure}
We apply this invariance in the case of the isometry (\ref{SpecialIsometry}), which repositions the point $b \in \partial \mathbb D$ to $1$ and the vertex at $z_j$ to the center of the disk. This enables us to compute the ratio
\begin{equation}
R_{j,n} \;=\; \frac{\psi_{\mu,1}(w(z_{j_n}))}{\psi_{\mu,1}(0)} \;=\;\psi_{\mu,1}\bigl(w_n\bigr)\,,
\end{equation}
where the complex numbers $w_n=w(z_{j_n})$ are once again the positions of the transformed nearest neighbors, uniformly distributed on a circle with radius $h$, as depicted in the right panel of Fig.~\ref{fig:taucalc}. Defining the complex phase
\begin{equation}
Z=e^{2\pi i/q}
\end{equation}
we can represent them as $w_n = hZ^{\tau_j+n}$, implying
\begin{equation}
\label{RnExplicit2}
R_{j,n} \;:=\;
\psi_{\mu,1}(hZ^{\tau_j+n})
\;=\;\left( \frac{\bigl|1-h Z^{\tau_j+n}\bigr|^2}{1-h^2} \right)^{\mu}\,.
\end{equation}
The fundamental assumption of this work, as noted in the main text, is that the correction factors $\chi_j$ can be solely expressed as a function of local inclination, i.e., $\chi_j = \chi(\tau_j)$. This transforms the eigenvalue equation on the lattice (\ref{EigenvalueProblem1}) into the following equation for the correction function $\chi(\tau)$:
\begin{equation}
\sum_{n=0}^{q-1}R_{j,n} \chi(\tau_{j_n}) \;=\; \bigl(q-\mathcal N \Lambda_\mu\bigr) \chi(\tau_j)\,.
\end{equation}
This equation must be valid at all vertices $j$ of the infinite lattice. Given that the corresponding inclinations $\tau_j$ appear to densely fill the interval $[0,1)$ across the lattice, we consider an arbitrary value $\tau\in[0,1)$ of some vertex as given and then compute the corresponding inclinations $\sigma_n(\tau)$ of the $q$ nearest neighbors, labeled by $n=0,\ldots,q-1$. These inclinations can be determined by mapping the neighbors isometrically to the center, employing techniques similar to those used in the previous section, leading to
\begin{equation}
\label{SigmaDef}
\sigma_n(\tau) \;=\; \left(\frac{1}{2\pi} \arg \left[ \Bigl( \frac{h-Z^{\tau+n}}{1-h Z^{\tau+n}} \Bigr)^q \right]\right) \mod 1\,,
\end{equation}
where $Z=e^{2\pi i/q}$. With
\begin{equation}
\label{RnExplicit}
R_n(\tau) \;=\; \biggl( \frac{\bigl|1-h Z^{\tau+n}\bigr|^2}{1-h^2} \biggr)^{\mu}
\end{equation}
this eventually leads to the equation
\begin{equation}
\label{DiffEq}
\sum_{n=0}^{q-1} R_n(\tau) \, \chi\bigl(\sigma_{n}(\tau)\bigr) \;=\; \bigl(q-\mathcal N \Lambda_\mu\bigr) \chi(\tau)
\end{equation}
which is expected to be valid for all $\tau \in [0,1)$. This equation links the function $\chi(\tau)$ linearly with the same function evaluated at $q$ different inclinations $\sigma_0(\tau),\ldots,\sigma_{q-1}(\tau)$ (see Fig.~\ref{supfig:neighbor-inclination}). Thus, it can be considered as a linear finite-difference equation for the function $\chi(\tau)$.

%=====================================================
\subsection{S4: Fourier Expansion of the Inclination Function}
\label{sec:S4}
%=====================================================
%
As detailed in the main text, our numerical results strongly suggest that it is advantageous to express the inclination function $\chi(\tau)$ as a Fourier series:
\begin{equation}
\label{FourierAnsatz2}
\chi(\tau) \;=\; \sum_{k=-\infty}^{+\infty} \gamma_k \, Z^{q\tau k}
\,,
\end{equation}
where $Z=e^{2\pi i/q}$, and the $\gamma_k$ are certain coefficients yet to be determined. Since eigenvectors are defined up to a factor, we are free to set $\gamma_0:=1$. In this section, we present technical specifics on deriving an eigenvalue problem for these coefficients.

To simplify the notations, let us introduce the abbreviation
\begin{equation}
Y_n := 1-h  Z ^{\tau+n}
\end{equation}
and its complex conjugate $\bar Y_n := 1-h  Z ^{-\tau-n}$, with $h$ defined in~(\ref{hdef2}). This enables us to rewrite Eqs.~(\ref{RnExplicit2}) and~(\ref{SigmaDef}) by
\begin{align}
R_n(\tau) \;&=\;\biggl( \frac{\bigl|1-h Z^{\tau+n}\bigr|^2}{1-h^2} \biggr)^{\mu}
\;=\; \frac{Y^\mu_n \bar Y^\mu_n}{(1-h^2)^{\mu}} \,,\\
Z^{q\sigma_{n}(\tau)} \;&=\;  \Bigl( \frac{h-Z^{\tau+n}}{1-h Z^{\tau+n}} \Bigr)^q
\;=\; \frac{(-)^{q}Z^{q\tau}\bar Y_n^q}{Y_n^q}
\,,
\end{align}
where we used $Z^{nq}=1$. Using the ansatz (\ref{FourierAnsatz2}), the difference equation~(\ref{DiffEq}) can then be reformulated as:
\begin{equation}
\sum_{n=0}^{q-1}
\frac{Y^\mu_n \bar Y^\mu_n}{(1-h^2)^{\mu}}
\sum_{k=-\infty}^{+\infty} \gamma_k \frac{(-1)^{qk}Z^{q\tau k}\bar Y_n^{qk}}{Y_n^{qk}}
\;=\; \bigl(q-\mathcal N \Lambda_\mu\bigr)
\sum_{k=-\infty}^{+\infty} \gamma_k Z^{q\tau k}\,.
\end{equation}
Organizing the terms yields:
\begin{equation}
\label{SEquation}
\frac{1}{(1-h^2)^{\mu}}
\sum_{k=-\infty}^{+\infty} \gamma_k
(-1)^{qk}Z^{q\tau k}
\underbrace{\sum_{n=0}^{q-1}
Y_n^{\mu-qk}
\bar Y_n^{\mu+qk}}_{=: S_k}
\;=\; \bigl(q-\mathcal N \Lambda_\mu\bigr)
\sum_{k=-\infty}^{+\infty} \gamma_k Z^{q\tau k}\,.
\end{equation}
We first evaluate the part enclosed in brackets
\begin{equation}
S_k   =\sum_{n=0}^{q-1} Y^{\mu-qk}_{n}\,\bar Y^{\mu+qk}_{n}\;=\;
 \sum_{l=0}^\infty \binom {\mu-qk} l
 \sum_{m=0}^\infty \binom {\mu+qk} m
 (-h)^{l+m}Z^{\tau(l-m)}\sum_{n=0}^{q-1}Z^{n(l-m)}
\end{equation}
where $\binom a b = \frac{\Gamma(a+1)}{\Gamma(b+1)\Gamma(a-b+1)}$. Given that $Z=e^{2\pi i/q}$, the last sum yields:
\begin{equation}
\sum_{n=0}^{q-1}Z^{n(l-m)} \;=\;
\begin{cases}
q & \hspace{3mm}\text{ if  } (l-m) \text{  is a multiple of } q \\
0 & \hspace{3mm}\text{ otherwise.}
\end{cases}
\end{equation}
The expression for $S_k$ therefore decomposes into three parts, namely, for $m=l$, for $m=l+qs$, and for $l=m+qs$ with $s \in \mathbb N$:
\begin{equation}
\begin{split}
S_k &= q \sum_{l=0}^\infty \binom {\mu-qk} l \binom {\mu+qk} l (-h)^{2l} \\
&+ q \sum_{s=1}^\infty \, \sum_{l=0}^\infty \binom {\mu-qk} l  \binom {\mu+qk} {l+qs} (-h)^{2l+qs}\, Z^{-\tau qs}\\
&+ q \sum_{s=1}^\infty \, \sum_{m=0}^\infty \binom {\mu-qk} {m+qs} \binom {\mu+qk} m (-h)^{2m+qs}\, Z^{\tau qs}
\end{split}
\end{equation}
It emerges that these sums can be expressed in terms of generalized hypergeometric functions:
\begin{equation}
\begin{split}
S_k &= q\,\, {}_2F_1(-\mu-qk,-\mu+qk;\,1;\,h^2) \\
&+ q \sum_{s=1}^\infty \,\binom {\mu+qk} {qs}\,\, {}_2F_1\bigl(-\mu+qk,-\mu+qs-qk;\,1+qs;\,h^2\bigr)  (-h)^{qs} Z^{-\tau qs}\\
&+ q \sum_{s=1}^\infty \,\binom {\mu-qk} {qs}\,\, {}_2F_1\bigl(-\mu-qk,-\mu+qs+qk;\,1+qs;\,h^2\bigr)  (-h)^{qs} Z^{\tau qs}
\end{split}
\end{equation}
Reinserting this expression back into Eq.~(\ref{SEquation}) and comparing the coefficients in the powers of $Z$ on both sides, it is straight-forward to show that the Fourier coefficients comply with the eigenvalue problem
\begin{equation}
\label{GammaEVP}
\sum_{k=-\infty}^{\infty} B_{j,k}\,\gamma_k \;=\; (q-\mathcal N \Lambda_\mu) \gamma_j
\end{equation}
for all $j \in \mathbb Z$, where the infinite-dimensional matrix $B_{j,k}$ is defined in terms of generalized hypergeometric functions as:
\begin{equation}
\label{matrixB}
B_{j,k} \;=\; \frac{q \,(-1)^{qj}\,h^{q|j-k|}}{(1-h^2)^\mu}
\begin{cases}
\binom{\mu-qk}{qj-qk}\,\,{}_2F_1\bigl(-\mu+qj,\,-\mu-qk;\,1+qj-qk;\,h^2\bigr) & \text{ if } j\geq k\\
\binom{\mu+qk}{qk-qj}\,\,{}_2F_1\bigl(-\mu-qj,\,-\mu+qk;\,1+qk-qj;\,h^2\bigr) & \text{ if } j<k
\end{cases}\,.
\end{equation}
Equivalently, we can rewrite this matrix in terms of generalized Jacobi functions $P_n^{\alpha,\beta}(z)$ as
\begin{equation}
\label{matrixB2}
B_{j,k} \;=\; \frac{q \,(-1)^{qj}\,h^{q|j-k|}}{(1-h^2)^\mu}
\begin{cases}
P_{\mu-qj}^{q(j-k),-1-2\mu}(1-2h^2) & \text{ if } j\geq k\\
P_{\mu+qj}^{q(k-j),-1-2\mu}(1-2h^2) & \text{ if } j<k
\end{cases}\,.
\end{equation}
Note that this matrix is symmetric under reflections
\begin{equation}
B_{j,k}=B_{-j,-k}.
\end{equation}
Thus, the eigenvectors of (\ref{GammaEVP}) are either symmetric or antisymmetric ($\gamma_j=\pm \gamma_{-j}$), corresponding to real-valued or purely imaginary correction functions. Given our interest in real-valued symmetric solutions with $\gamma_j= \gamma_{-j}$, we can further condense the eigenvalue problem to:
\begin{equation}
\label{GammaEVPSymmetric}
\sum_{k=0}^{\infty} C_{j,k}\,\gamma_k \;=\; (q-\mathcal N \Lambda) \gamma_j
\end{equation}
for $j\geq 0$ with
\begin{equation}
C_{j,k} :=
\begin{cases}
B_{j,0} & \text{ if } k=0 \\
B_{j,k}+B_{j,-k} & \text{ if } k>0
\end{cases}
\end{equation}
%
%=====================================================
\subsection{S5: Analytical Solutions for $\mu \in \mathbb N$}
\label{sec:S5}
%=====================================================
%
For $\mu \in \mathbb N$, the matrix $B$ appears to possess a block structure. More specifically, if $sq\leq \mu < (s+1)q$ for $s \in \mathbb N$, we find that:
\begin{itemize}
  \setlength\itemsep{0em}
  \setlength{\itemindent}{1cm}
\item $B_{j,k}=0$ if $j>s$ and $k\leq s$
\item $B_{j,k}=0$ if $j<-s$ and $k\geq -s$
\item $B_{j,k}\neq0$ otherwise
\end{itemize}
In this case, the matrix exhibits a block structure that allows us to determine the eigenvector only within the block. This means that we can truncate $B$ to a $(2s+1)\times(2s+1)$ matrix with indices in the range $|j|\leq s$ and $|k| \leq s$. This enables us to solve the corresponding eigenvalue problem exclusively within this block and to set all remaining Fourier coefficients $\gamma_k$ with $|k|>s$ to zero.

For $\mu=0,1,\ldots,q-1$ where $s=0$, we obtain a one-dimensional block matrix with the trivial eigenvector $\gamma_0=1$ and the eigenvalue:
\begin{equation}
 \Lambda^{[s=0]}_\mu =  \frac{q}{\mathcal N}\Bigl( 1-\frac{1}{(1-h^2)^\mu} {}_2F_1(-\mu,-\mu;\, 1;\,h^2) \Bigr)\,.
\end{equation}
This replicates our earlier result where the lattice eigenfunction aligns with the continuum eigenfunction.

For the next group of integer values $\mu=q,q+1,\ldots,2q-1$, where $s=1$, we attain a $3\times 3$ matrix $B$ (or equivalently a $2\times 2$ matrix $C$) which can be exactly diagonalized. Here, we find the following explicit exact solution
\begin{equation}
\Psi_{\mu,b}(z_j) \;=\; \, \Bigl( 1+2\gamma_1\cos(2\pi \tau_j) \Bigr) \,\psi_{\mu,b}(z_j)
\end{equation}
with the Fourier coefficient
\begin{small}
\begin{equation}
\gamma_1 =\frac{2 (-1)^q h^q \binom{\mu }{q} \, _2F_1\left(q-\mu ,-\mu ;q+1;h^2\right)}{-(-1)^q \left(h^{2 q} \binom{q+\mu }{2 q} \, _2F_1\left(q-\mu ,q-\mu ;2
   q+1;h^2\right)+\, _2F_1\left(-q-\mu ,q-\mu ;1;h^2\right)\right)+\, _2F_1\left(-\mu ,-\mu ;1;h^2\right)+\sqrt{W}}
\end{equation}
\end{small}
and the eigenvalue
\begin{small}
\begin{equation}
\begin{split}
\mathcal N \Lambda^{[s=1]}_\mu \;=\; q \,-\,
\frac{1}{2} q \left(1-h^2\right)^{-\mu } \Bigl(
&-(-1)^q h^{2 q} \binom{q+\mu }{2 q} \, _2F_1\left(q-\mu ,q-\mu ;2 q+1;h^2\right)\\
&-\, _2F_1\left(-\mu ,-\mu ;1;h^2\right)-(-1)^q
   \, _2F_1\left(-q-\mu ,q-\mu ;1;h^2\right)+2 \left(1-h^2\right)^{\mu }-\sqrt{W}\Bigr)\,,
\end{split}
\end{equation}
\end{small}
where
\begin{small}
\begin{equation}
\begin{split}
W \;=\;& \left(1-h^2\right)^{4 \mu +2} \left[8 (-1)^q h^{2 q} \binom{\mu }{q} \binom{q+\mu }{q} \, _2F_1\left(\mu +1,q+\mu +1;q+1;h^2\right)^2+\, _2F_1\left(\mu +1,\mu
   +1;1;h^2\right)^2\right)
   \\&+(-1)^{2 q} \left(h^{2 q} \binom{q+\mu }{2 q} \, _2F_1\left(q-\mu ,q-\mu ;2 q+1;h^2\right)+\, _2F_1\left(-q-\mu ,q-\mu
   ;1;h^2\right)\right)^2\\
   &-2 (-1)^q \, _2F_1\left(-\mu ,-\mu ;1;h^2\right) \left(h^{2 q} \binom{q+\mu }{2 q} \, _2F_1\left(q-\mu ,q-\mu ;2 q+1;h^2\right)+\,
   _2F_1\left(-q-\mu ,q-\mu ;1;h^2\right)\right]
\end{split}
\end{equation}
\end{small}
Note that this nontrivial solution is exact across the entire infinite hyperbolic lattice.

%=====================================================
\subsection{S6: Radial Eigenmodes on the Infinite Lattice}
\label{sec:S6}
%=====================================================
%
Upon calculating the plane-wave eigenfunctions $\Psi_{\mu,b}(z_j)$, we can compute the corresponding radial eigenfunctions on the hyperbolic tiling by performing a Fourier transform in the angle $\beta$, which defines the location of the source $b=e^{i\beta}$ on the boundary:
\begin{equation}
U_{\mu}^m(z_j)\;=\;\frac{1}{2\pi}\int_0^{2\pi} \textrm{d} \beta \, e^{i m \beta}\,\Psi_{\mu,e^{i\beta}}(z_j)\,.
\end{equation}
As all plane-wave eigenfunctions
\begin{equation}
\Psi_{\mu,b}(z_j)\;=\;\psi_{\mu,b}(z_j)\chi(\tau_j)\;=\;
\psi_{\mu,b}(z_j)
\sum_{k=-\infty}^{\infty}\gamma_k\,Z^{q \tau_j k}
\end{equation}
correspond to the same eigenvalue $\Lambda_\mu$ regardless of $\beta$, their linear combination is also an eigenfunction of the eigenvalue $\Lambda_\mu$. Setting $b=e^{i\beta}$ and inserting Eqs.(\ref{ContinuumEigenfunction}) and(\ref{inclinationRelation}), i.e.,
\begin{align}
\psi_{\mu,b}(z_j)
\;&=\; \Bigl( \frac{|b-z_j|^2}{1-|z_j|^2} \Bigr)^{\mu}
\;=\;  \Bigl( \frac{|1-\overline b z_j|^2}{1-|z_j|^2} \Bigr)^{\mu}
\\
Z^{q \tau_j}\;&=\;
e^{2\pi i \tau_j} \;=\;
\Bigl( \frac 1 h \, \frac{(1-b \overline z_j)(z'_j-z_j)}{(b-z_j)(1-z'_j\overline z_j)} \Bigr)^q\,,
\end{align}
we obtain
\begin{equation}
U_{\mu}^m(z_j)\;=\;\frac{1}{2\pi}\int_0^{2\pi} e^{i m \beta}\,
 \left( \frac{|1-\overline b z_j|^2}{1-|z_j|^2} \right)^{\mu}\,
 \sum_{k=-\infty}^{\infty}\gamma_k\,
 \left( \frac 1 h \, \frac{(1-\overline z_jb)(z'_j-z_j)}{(b-z_j)(1-z'_j\overline z_j)} \right)^{qk}\,,
\end{equation}
where, as before, $z'_j$ denotes the position of one of the nearest neighbors of $z_j$. Organizing the terms yields
\begin{equation}
\begin{split}
\label{radlet1}
U_\mu^{m}(z_j) \;&=\;\frac{1}{2\pi (1-|z_j|^2)^\mu}\,
\sum_{k=-\infty}^\infty \gamma_k \,
\frac{(z'_j-z_j)^{qk}}{h^{qk} (1-z'_j \bar z_j)^{qk}}
\underbrace{\int_0^{2\pi}\text{d}\beta\,
b^{m-qk}\,
\frac{(|1-\overline b z_j|^2)^\mu\,(1-b\bar z_j)^{qk}}{(1-\overline b z_j)^{qk}}}_{=:\,I_{k,m}\,\,\text{to be evaluated}}
\end{split}
\end{equation}
First, we compute the integral $I_{k,m}$ indicated by the curly bracket. Substituting $b \overline z_j = |z_j| e^{i \alpha}$ transforms the integral into
\begin{equation}
I_{k,m}\,
\;=\; \Bigl( \frac{|z_j|}{\overline z_j} \Bigr)^{m-qk}
\int_0^{2\pi}\text{d}\alpha\,(e^{i \alpha})^{m-qk} (1-|z_j| e^{i \alpha})^{\mu+qk}\,(1-|z_j| e^{-i \alpha})^{\mu-qk}
\end{equation}
Expanding the powers as generalized binomials with coefficients $\binom a b = \frac{\Gamma(a+1)}{\Gamma(b+1)\Gamma(a-b+1)}$ we get
\begin{equation}
\begin{split}
I_{k,m}\, \;=\; \; & \Bigl( \frac{|z_j|}{\overline z_j} \Bigr)^{m-qk}
\int_0^{2\pi}\text{d}\alpha\,(e^{i \alpha})^{m-qk}
\sum_{l,s=0}^{\infty}\binom{\mu+qk}{l}\binom{\mu-qk}{s}
(-|z_j|  e^{i \alpha})^l (-|z_j| e^{-i \alpha})^s \\
\;=\; &
\Bigl( \frac{|z_j|}{\overline z_j} \Bigr)^{m-qk}
\sum_{l,s=0}^{\infty}\binom{\mu+qk}{l}\binom{\mu-qk}{s}
(-|z_j|)^{l+s}
\underbrace{\int_0^{2\pi}\text{d}\alpha\,e^{i\alpha(m-qk+l-s)}}_{=2\pi \delta_{s,m+l-qk}}\\
\;=\; &
2\pi\Bigl( \frac{|z_j|}{\overline z_j} \Bigr)^{m-qk}
\sum_{l=\max(0,qk-m)}^{\infty}\binom{\mu+qk}{l}\binom{\mu-qk}{m+l-qk}
(-|z_j|)^{2l+m-qk}\\
\;=\; &
2\pi\Bigl( -\frac{|z_j|}{\overline z_j} \Bigr)^{m-qk}
\begin{cases}
|z_j|^{m-q k}\binom{\mu-q k}{m-q k}\, {}_2F_1(m-\mu,-\mu-q k;\,1+m-q k;\,|z_j|^2) & \text{ if } m \geq q k \\
|z_j|^{-m+q k}\binom{\mu+q k}{-m+q k}\, {}_2F_1(-m-\mu,-\mu+q k;\,1-m+q k;\,|z_j|^2) & \text{ if } m < q k
\end{cases}
\\
\;=\; &
2\pi
\begin{cases}
(-z_j)^{m-q k}\binom{\mu-q k}{m-q k}\, {}_2F_1(m-\mu,-\mu-q k;\,1+m-q k;\,|z_j|^2) & \text{ if } m \geq q k \\
(-\overline z_j)^{-m+q k}\binom{\mu+q k}{-m+q k}\, {}_2F_1(-m-\mu,-\mu+q k;\,1-m+q k;\,|z_j|^2) & \text{ if } m < q k \\
\end{cases}
\end{split}
\end{equation}
where ${}_2F_1$ denotes once again the generalized hypergeometric function.
Inserting this result for $I_{k,m}$ back into~(\ref{radlet1})
\begin{equation}
U_\mu^{m}(z_j)\;=\;\frac{1}{2\pi (1-|z_j|^2)^\mu}\,
\sum_{k=-\infty}^\infty \gamma_k \,
\frac{(z'_j-z_j)^{qk}}{h^{qk} (1-z'_j \bar z_j)^{qk}} \; I_{k,m}
\end{equation}
provides the final result for the radial eigenfunction
\begin{small}
\label{RadialFinal}
\begin{equation}
U_\mu^{m}(z_j) \;=\; \frac{1}{(1-|z_j|^2)^\mu}\,
\sum_{k=-\infty}^\infty \gamma_k
\left[ \frac{z_j-z'_j}{h\,(1-z'_j \bar z_j)} \right]^{qk}
\begin{cases}
z_j^{m-q k}\binom{\mu-q k}{m-q k}\, {}_2F_1\bigl(m-\mu,-\mu-q k;\,1+m-q k;\,|z_j|^2\bigr) & \text{ if } m \geq q k \\
\overline z_j^{q k-m}\binom{\mu+q k}{q k-m}\, {}_2F_1\bigl(-m-\mu,-\mu+q k;\,1-m+q k;\,|z_j|^2\bigr) & \text{ if } m < q k \\
\end{cases}
\end{equation}
\end{small}
\paragraph{Special cases:}
For $\mu=0,1,\ldots,q-1$, where only the term $k=0$ contributes, this expression simplifies to
\begin{equation}
\begin{split}
u_\mu^{m}(z_j) \;&=\;
 \frac{1}{(1-|z_j|^2)^\mu}\,
\begin{cases}
z_j^{m}\binom{\mu}{m}\, {}_2F_1\bigl(m-\mu,-\mu;\,1+m;\,|z_j|^2\bigr) & \text{ if } m \geq 0 \\
\overline z_j^{-m}\binom{\mu}{-m}\, {}_2F_1\bigl(-m-\mu,-\mu;\,1-m;\,|z_j|^2\bigr) & \text{ if } m < 0 \\
\end{cases}\\
\;&=\;\Gamma(\mu+1)
\begin{cases}
z_j^{m} \frac{(-|z_j|^2)^{-m/2}}{\Gamma(\mu-m+1)} P_\mu^{-m}\Bigl( \frac{1+|z_j|^2}{1-|z_j|^2} \Bigr)& \text{ if } m \geq 0 \\
\overline z_j^{-m} \frac{(-|z_j|^2)^{m/2}}{\Gamma(\mu+m+1)} P_\mu^{m}\Bigl( \frac{1+|z_j|^2}{1-|z_j|^2} \Bigr)& \text{ if } m < 0 \\
\end{cases}
\end{split}
\end{equation}
and one can show that this expression consistently reduces to the known radial eigenfunction in the continuum case
\begin{equation}
u_{\mu}^m(z_j) \;\propto\; e^{i m \phi_j} P^m_{-\mu-1}\Bigl( \frac{1+r_j^2}{1-r_j^2} \Bigr)\,,
\end{equation}
where $z_j=r_je^{i\phi_j}$.

%=====================================================
\subsection{S7: Numerical Data}
\label{sec:S7}
%=====================================================
%

\begin{table}[h]\label{tab:eigenvalues}
\begin{center}

\begin{tabular}{c||c|c|c}
 $\mu$ & $\{3,7\}$ & $\{3,8\}$ & $\{4,8\}$ \\ %[0.5ex]
 \hline\hline
 $-0.5$ & $1.127627$ & $1.245405$ & $1.548876$ \\
 \hline
 $-0.25$ & $0.849605$ & $0.942441$ & $1.194023$ \\
 \hline
 $0.25$ & $-1.468768$ & $-1.686357$ & $-2.402387$ \\
 \hline
 $0.5$ & $-3.639259$ & $-4.304511$ & $-6.726293$ \\
 \hline
 $1$ & $-10.62388$ & $-13.65685$ & $-27.31370$ \\
 \hline
 $7$ & $-7.465861\times10^3$ & $-9.207830\times10^4$ & $-3.302949\times10^7$ \\
 \hline
 $8$ & $-2.083553\times10^4$ & $-3.980441\times10^5$ & $-3.583152\times10^8$ \\
 \hline \hline
 $h$            & $0.4969704$ & $0.6435943$ & $0.8408964$ \\
 \hline
 $\mathcal N$   & $0.4322143$ & $0.8284271$ & $1.4142136$
\end{tabular}
\end{center}
\caption{Numerical eigenvalues $\Lambda_\mu$ as well as the parameters $h$ and $\mathcal N$ for three different $\{p,q\}$-lattices. The numerical precision is $\pm 1$ in the last digit.}
\end{table}

\begin{table}[h]\label{tab:fouriercoefficients}
\begin{center}

\begin{tabular}{c||c|c|c|c|c|c}
  & \multicolumn{2}{|c}{$\{3,7\}$} & \multicolumn{2}{|c}{$\{3,8\}$} & \multicolumn{2}{|c}{$\{4,8\}$}\\
 \hline
 $\mu$  & $\Lambda$ & $\left\{ \gamma_k \right\}$ & $\Lambda$ & $\left\{ \gamma_k \right\}$ & $\Lambda$ & $\left\{ \gamma_k \right\}$\\
 \hline\hline
 $1$ & $-10.6239$ & $\left\{1\right\}$ & $-13.6569$ & $\left\{1\right\}$ & $-27.3137$ & $\left\{1\right\}$\\
 \hline
 %$2$ & $-42.3251$ & $\left\{1\right\}$ & $-69.9411$ & $\left\{1\right\}$ & $XXX$ & $\left\{1\right\}$\\
 %\hline
 %$3$ & $-127.439$ & $\left\{1\right\}$ & $-295.078$ & $\left\{1\right\}$ & $XXX$ & $\left\{1\right\}$\\
 %\hline
 %$4$ & $-356.16$ & $\left\{1\right\}$ & $-1.21811\times 10^3$ & $\left\{1\right\}$ & $XXX$ & $\left\{1\right\}$\\
 %\hline
 %$5$ & $-978.794$ & $\left\{1\right\}$ & $-5.08193\times 10^3$ & $\left\{1\right\}$ & $XXX$ & $\left\{1\right\}$\\
 %\hline
 $6$ & $-2.69424\times 10^3$ & $\left\{1\right\}$ & $-2.15029\times 10^4$ & $\left\{1\right\}$ & $-3.07439\times 10^6$ & $\left\{1\right\}$\\
 \hline
 $7$ & $-7.46586\times 10^3$ & $\left\{1,-1.16212\times 10^{-4}\right\}$ & $-9.20783\times 10^4$ & $\left\{1\right\}$ & $-3.30295\times 10^7$ & $\left\{1\right\}$\\
 \hline
 $8$ & $-2.08355\times 10^4$ & $\left\{1,-5.41973\times 10^{-4}\right\}$ & $-3.98044\times 10^5$ & $\left\{1,-5.15986\times 10^{-5}\right\}$ & $-3.58315\times 10^8$ & $\left\{1,-7.2897\times 10^{-5}\right\}$\\
 \hline
 %$9$ & $-5.8503\times 10^4$ & $\left\{1,-1.46461\times 10^{-3}\right\}$ & $-1.73383\times 10^6$ & $\left\{1,-2.58365\times 10^{-4}\right\}$ & $XXX$ & $\left\{1\right\}$\\
 %\hline
 %$15$ & $-3.07885\times 10^7$ & $\left\{1,-2.09637\times10^{-2},-3.93026\times10^{-8}\right\}$ & $-3.98044\times 10^5$ & $\left\{1,-5.15986\times 10^{-5}\right\}$ & $-3.98044\times 10^5$ & $\left\{1,-5.15986\times 10^{-5}\right\}$\\
 \hline
\end{tabular}
\end{center}
\caption{Analytical eigenvalues $\Lambda_\mu$ and Fourier-coefficients $\gamma_k$ for three different $\{p,q\}$-lattices. The output is rounded to the last digit.}

\end{table}

\begin{figure}[ht]
\includegraphics[width=85mm]{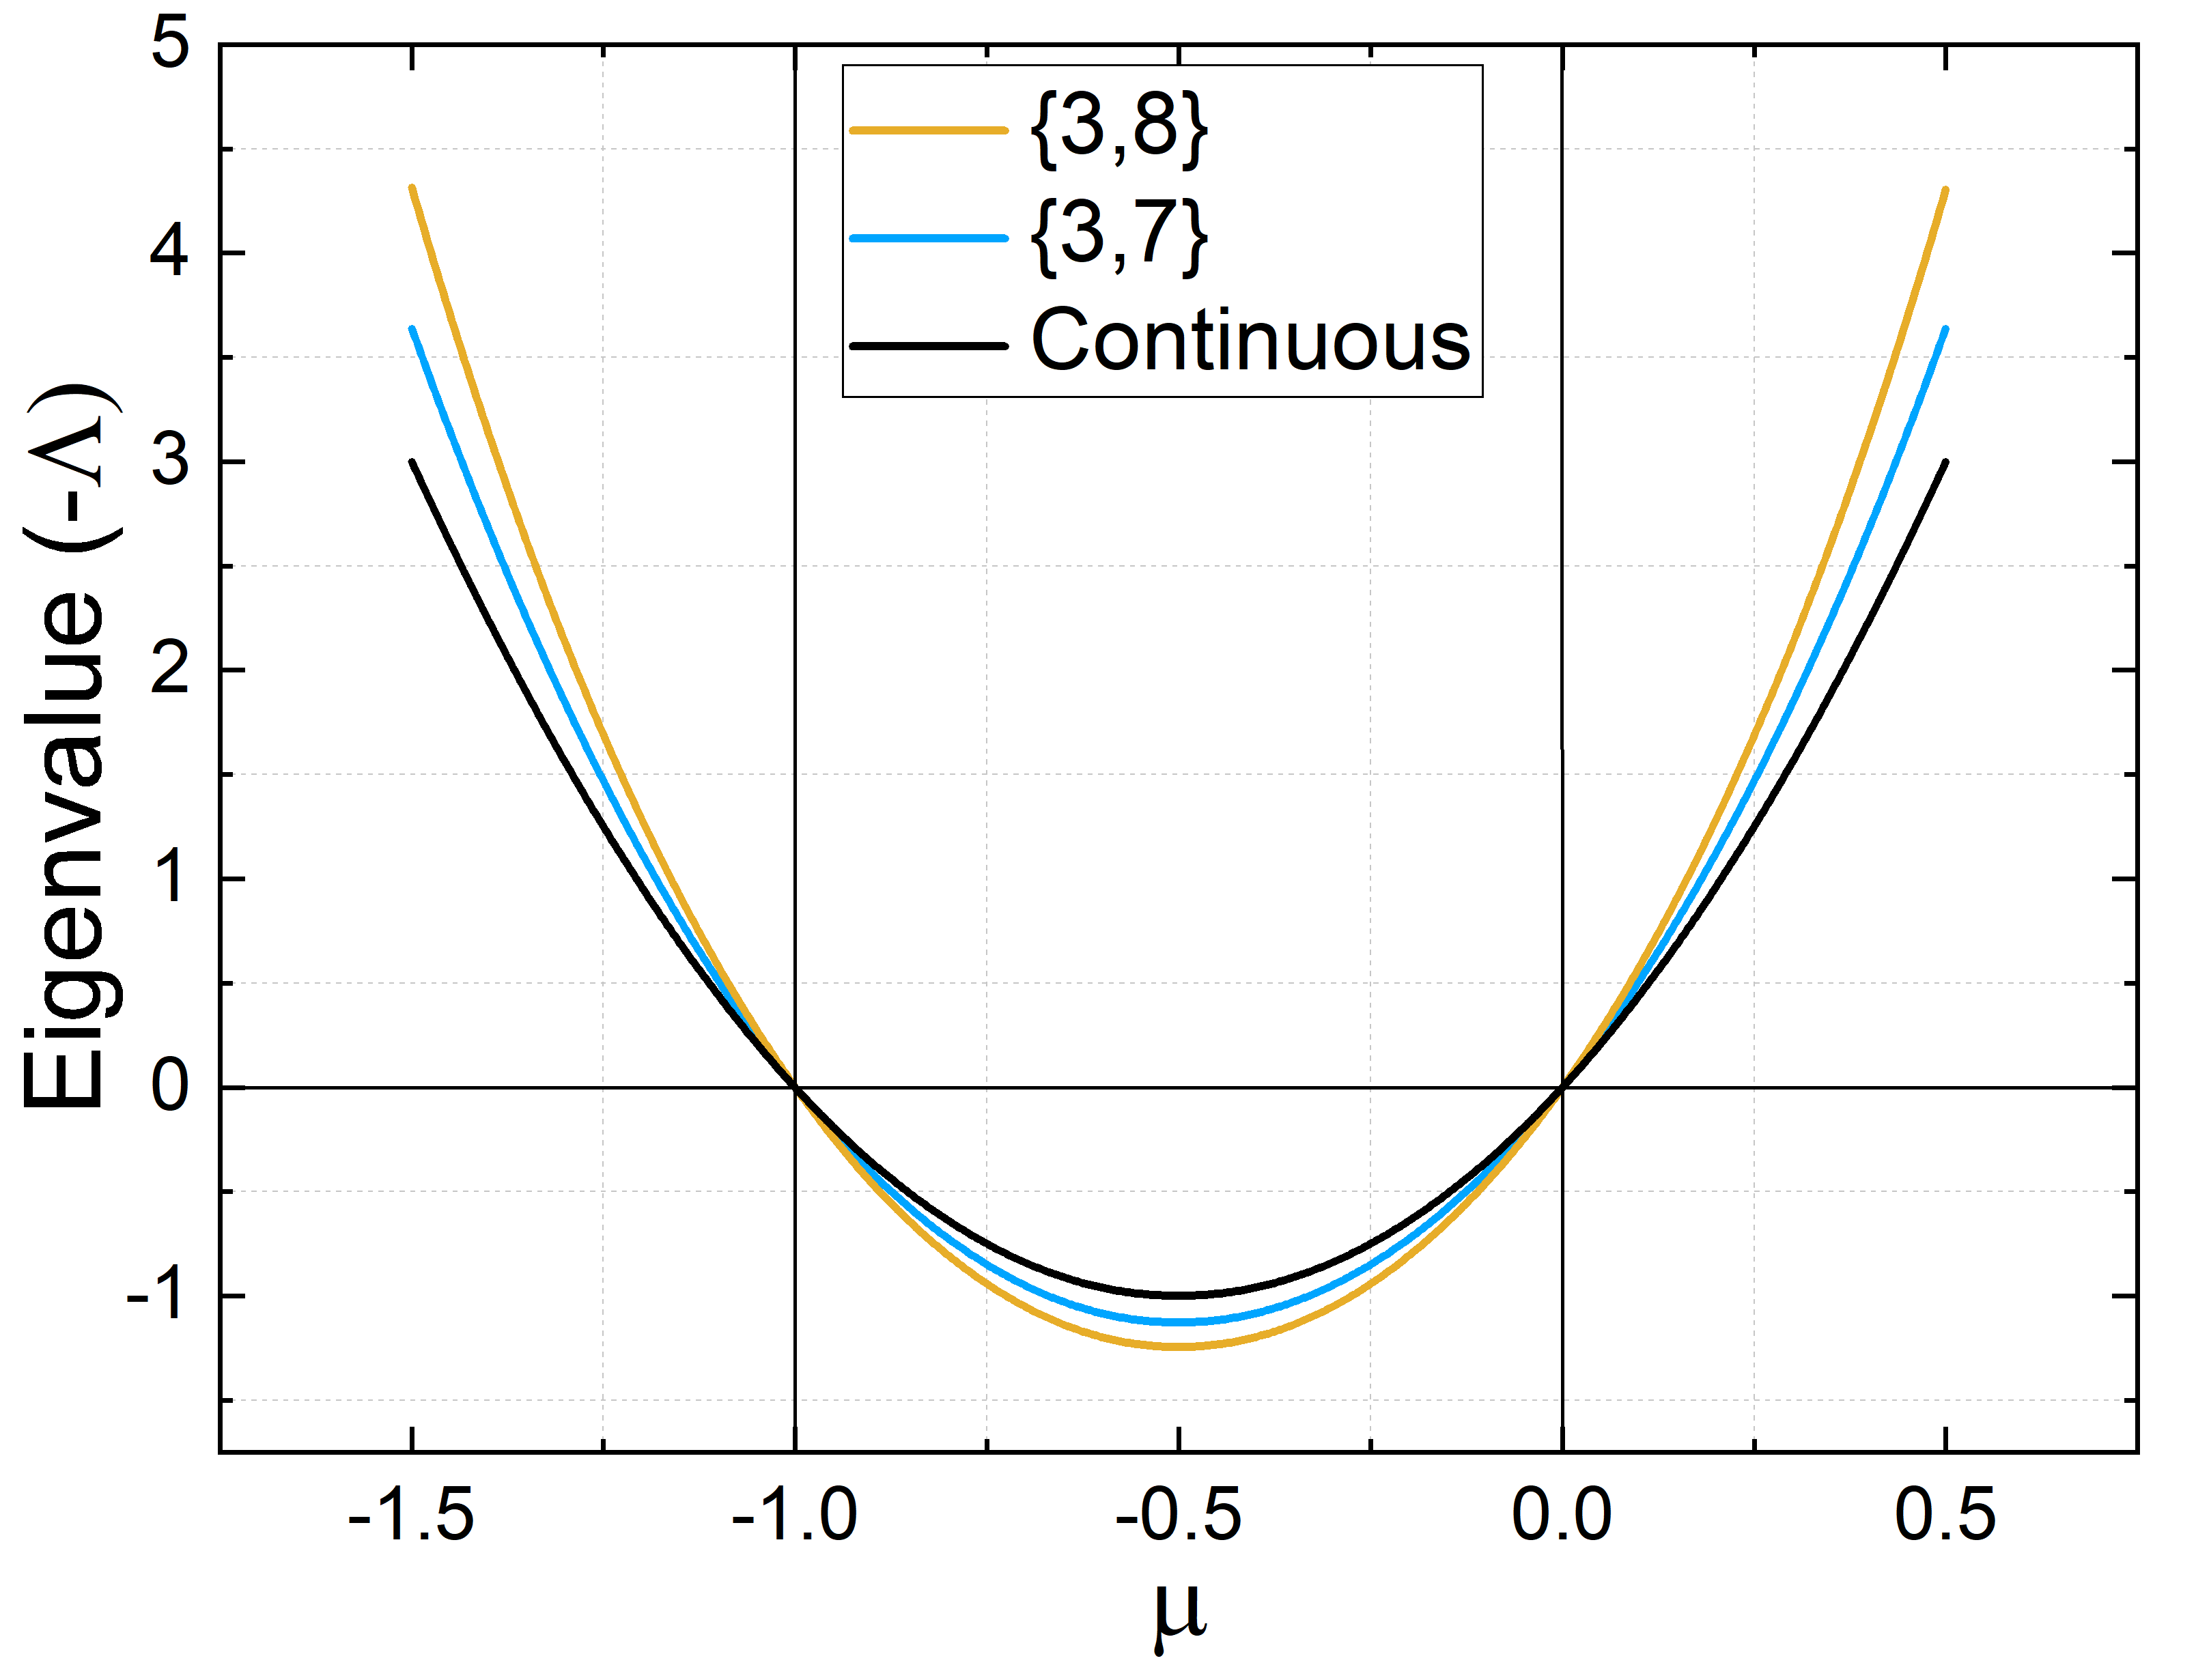}
\caption{
\label{fig:numericaleigenvalues}
Numerically determined dispersion relation of the eigenvalue $-\Lambda_\mu$ on a $\{3,7\}$ and $\{3,8\}$ lattice compared to the continuous solution. Note the expected zeros for $\mu= -1,0$ and the minimum at $\mu=-0.5$.
}
\end{figure}

% \begin{figure}[t]
% \includegraphics[width=\linewidth]{figures/eigen73.png}
% \caption{Caption placeholder. Note: Wahrscheinlich lieber ins supplement.}
% \end{figure}
%
